# Supplementary material for: Detecting Dispersed Radio Transients in Real Time Using Convolutional Neural Networks
Source: arXiv:2103.15418 source file (2021-08-06)
Supplement: Supplementary file 1 [file extra_examples.tex]

\section{Additional Dispersed Bursts from Real Data}
\label{sec:supp_additional_candidates}
\begin{center}
    \captionsetup{type=figure}
    \includegraphics[width=0.45\linewidth]{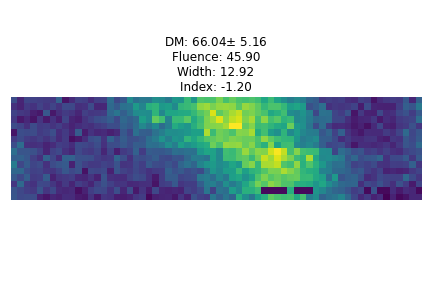}
    \includegraphics[width=0.45\linewidth]{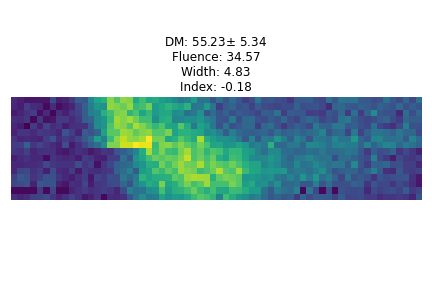}
    \includegraphics[width=0.45\linewidth]{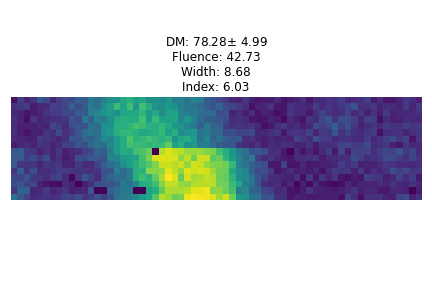}
    \includegraphics[width=0.45\linewidth]{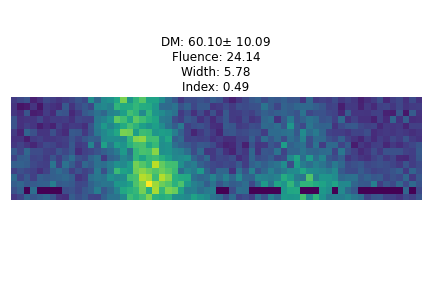} \\
    \includegraphics[width=0.45\linewidth]{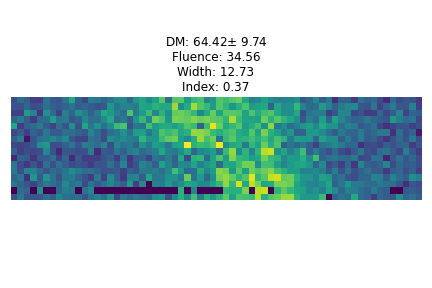}
    \includegraphics[width=0.45\linewidth]{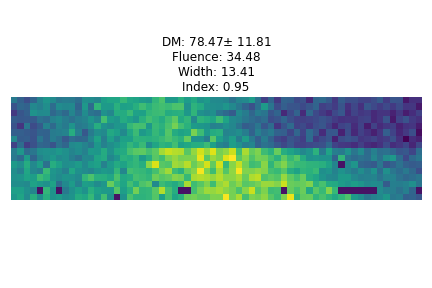}
    \includegraphics[width=0.45\linewidth]{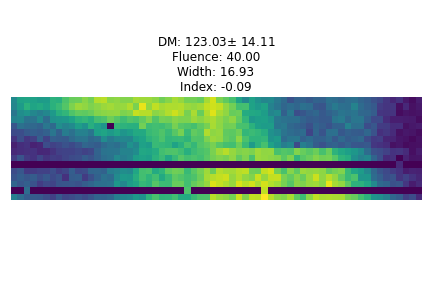}
    \includegraphics[width=0.45\linewidth]{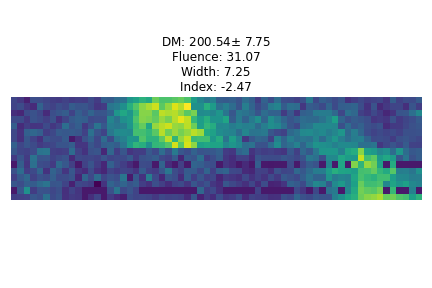}
    \caption{Transient candidates from a 5-hour survey on 2019-09-01 18:55 along with their inferred parameters $\hat{\bm \theta}$.}
    \label{fig:2019data}
\end{center}
In \cref{fig:2019data} we show some additional examples of dispersed candidates that were found in test runs of our methods on AARTFAAC data.
These were obtained from a 5-hour survey on 2019-09-01 18:55.
Included are the inferred parameters $\hat{\bm \theta}$ (dispersion measure DM, fluence, width, and spectral index) that the neural network infers.
