# Supplementary material for: Detecting Dispersed Radio Transients in Real Time Using Convolutional Neural Networks
Source: arXiv:2103.15418 source file (2021-08-06)
Supplement: Supplementary file 2 [file transient_examples.tex]

\section{Examples of simulated dispersed transients}
In \cref{fig:simulated_transient_examples} we depict examples of the simulated transients used to train the convolutional neural network.
We also provide the parameters $\bm \theta$ (dispersion measure DM, fluence, width, spectral index and reference time $t_0$) that were used to simulate them.
\label{sec:supp_simualted_transients}
\begin{figure*}[ht]
    \centering
    \includegraphics[width=\linewidth]{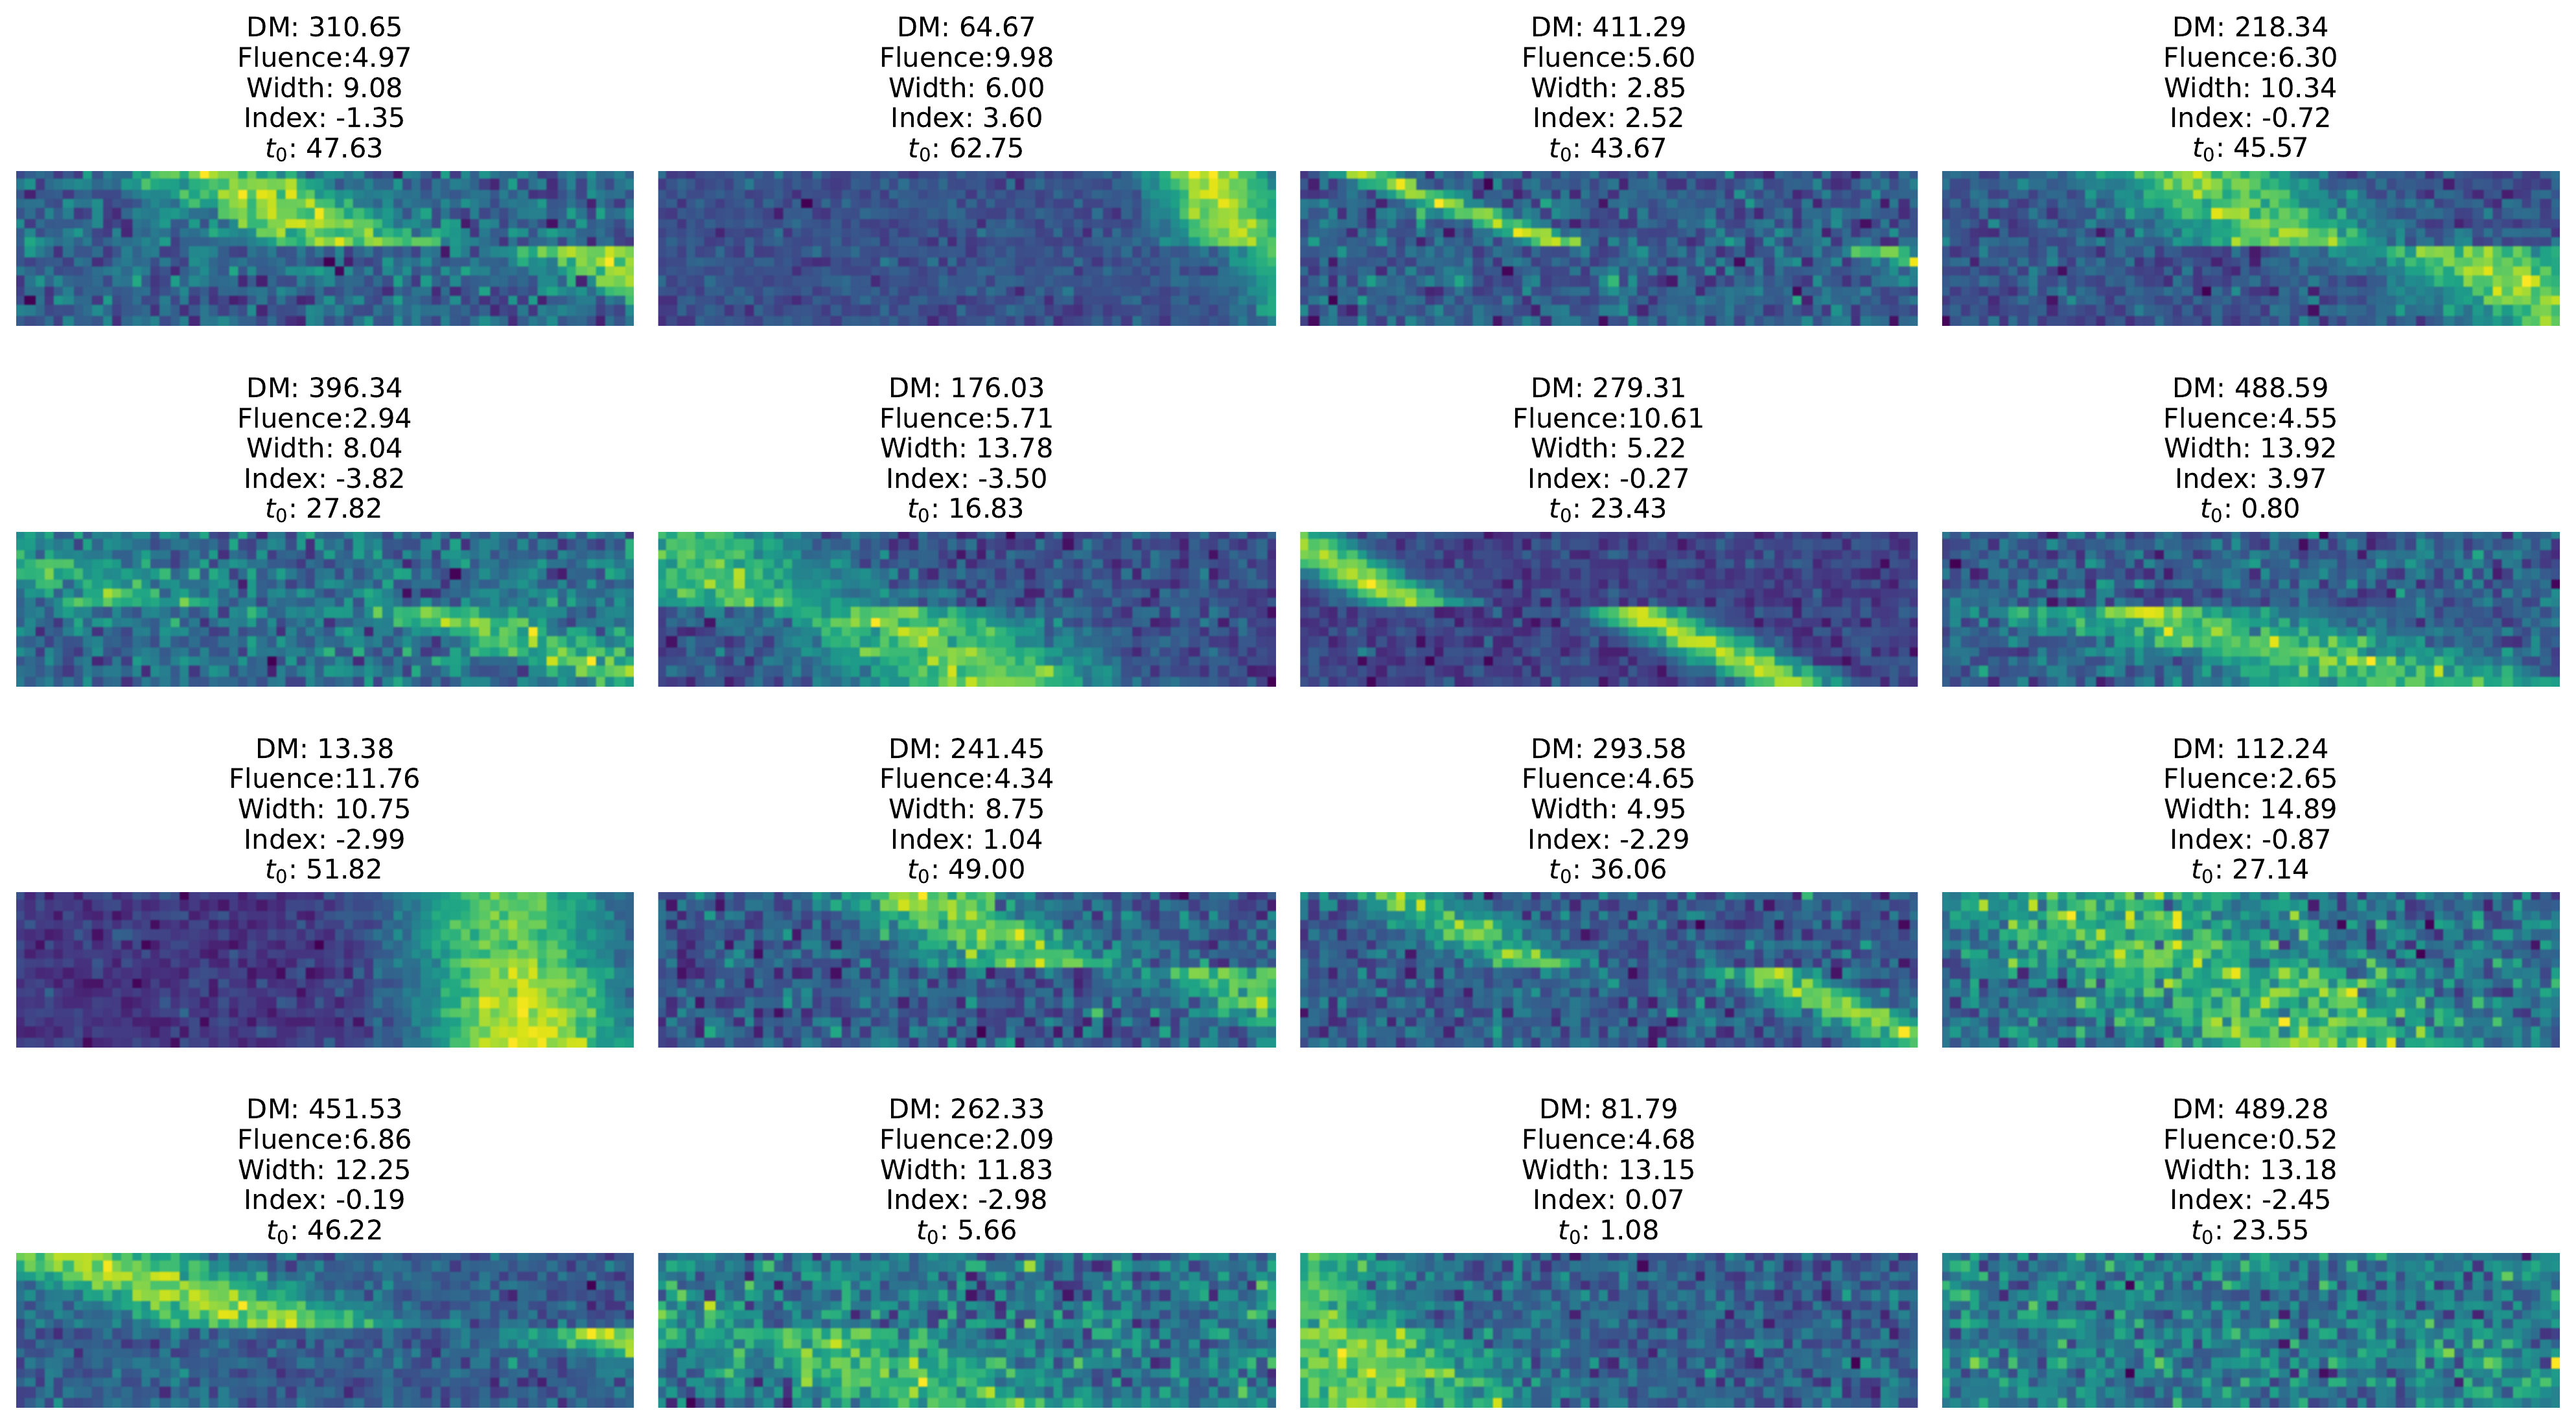}
    \caption{Selection of simulated dispersed transients. Above the dynamic spectra the parameters $\bm \theta$ that were used to simulate the example are shown.}
    \label{fig:simulated_transient_examples}
\end{figure*}
